# Supplementary material for: Spectroscopic factors in dripline nuclei
Source: arXiv:2107.12160 source file (2021-12-03)
Supplement: Supplementary file 1 [file Supplement.pdf]

# Supplemental Material for "Spectroscopic factors in dripline nuclei"

J. Wylie,[1,2] J. Okołowicz,[3] W. Nazarewicz,[1,2] M. Płoszajczak,[4]
S.M. Wang (王思敏),[1,5] X. Mao (毛兴泽),[1,2] and N. Michel[6,7]

[1] *FRIB/NSCL Laboratory, Michigan State University, East Lansing, Michigan 48824, USA*
[2] *Department of Physics and Astronomy, Michigan State University, East Lansing, Michigan 48824, USA*
[3] *Institute of Nuclear Physics, Polish Academy of Sciences, Radzikowskiego 152, PL-31342 Kraków, Poland*
[4] *Grand Accélérateur National d'Ions Lourds (GANIL), CEA/DSM - CNRS/IN2P3, BP 55027, F-14076 Caen Cedex, France*
[5] *Institute of Modern Physics, Fudan University, Shanghai 200433, China*
[6] *Institute of Modern Physics, Chinese Academy of Sciences, Lanzhou 730000, China*
[7] *School of Nuclear Science and Technology, University of Chinese Academy of Sciences, Beijing 100049, China*
(Dated: Received 22 July 2021; revised 31 August 2021; accepted 16 November 2021; published 3 December 2021)

This supplemental material contains supplemental discussion of the binding energies and spectra of $A = 8{,}9$ dripline nuclei obtained in our GSM calculations, non-resonant structure of the spectroscopic factor $\mathcal{S}^2_{p_{3/2}}$, and the tables of dominant GSM configurations.

## S.I. Spectra of mirror threshold $A = 8{,}9$ nuclei

Figure S1 shows the binding energies and spectra of $A = 8{,}9$ dripline nuclei obtained in our GSM calculations. On the proton-rich side, $^{8}$C is proton-unstable, $^{8}$B is a proton halo ($S_p = 136\,\mathrm{keV}$) [1, 2], and $^{9}$C has $S_p = 1.3\,\mathrm{MeV}$. The mirror neutron-rich nuclei $^{8}$He/$^{8,9}$Li are all neutron-bound. Here, the extremely neutron-rich $^{8}$He is a four-neutron halo. It is seen that the energy levels of mirror nuclei are reproduced fairly well, which suggest that the Coulomb energy displacement and the Thomas-Ehrman shift are under control in the GSM model.

## S.II. Non-resonant contributions to the spectroscopic factor

The squared spectroscopic amplitudes $\mathcal{A}^2_{p_{3/2}}(k_p)$ of the non-resonant states contributing to the spectroscopic factor $\mathcal{S}^2_{p_{3/2}}$ are shown in Fig. S2. The value of the SF is primarily determined by the contribution from the $0p_{3/2}$ bound pole.

[1] R. E. Warner, J. H. Kelley, P. Zecher, F. D. Becchetti, J. A. Brown, C. L. Carpenter, A. Galonsky, J. Kruse, A. Muthukrishnan, A. Nadasen, R. M. Ronningen, P. Schwandt, B. M. Sherrill, J. Wang, and J. S. Winfield, "Evidence for a proton halo in $^{8}$B: Enhanced total reaction cross sections at 20 to 60 mev/nucleon," Phys. Rev. C **52**, R1166–R1170 (1995).

[2] G. Korolev, A. Dobrovolsky, A. Inglessi, G. Alkhazov, P. Egelhof, A. Estradé, I. Dillmann, F. Farinon, H. Geissel, S. Ilieva, Y. Ke, A. Khanzadeev, O. Kiselev, J. Kurcewicz, X. Le, Y. Litvinov, G. Petrov, A. Prochazka, C. Scheidenberger, L. Sergeev, H. Simon, M. Takechi, S. Tang, V. Volkov, A. Vorobyov, H. Weick, and V. Yatsoura, "Halo structure of $^{8}$B determined from intermediate energy proton elastic scattering in inverse kinematics," Phys. Lett. B **780**, 200–204 (2018).

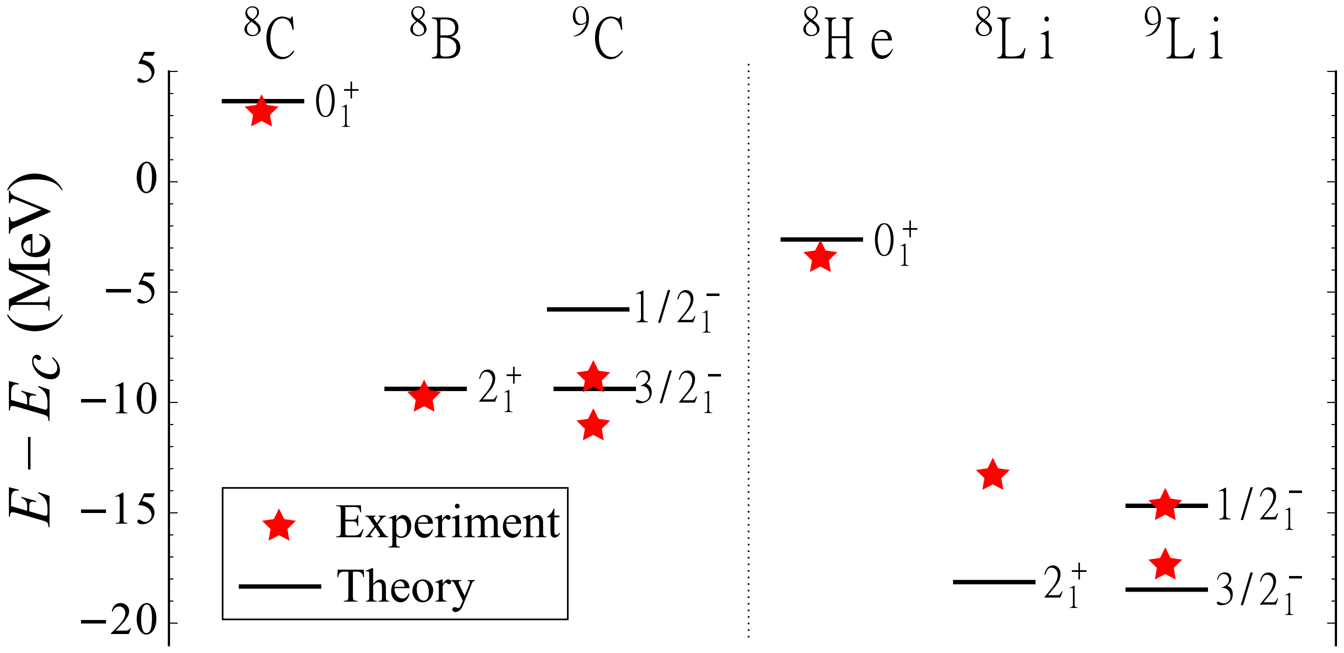


FIG. S1. GSM spectra of proton-rich nuclei $^{8,9}$C and $^{8}$B (left) and their neutron-rich mirror partners $^{8}$He/$^{8,9}$Li (right) compared to experiment. Energies are shown with respect to the $^{4}$He core.

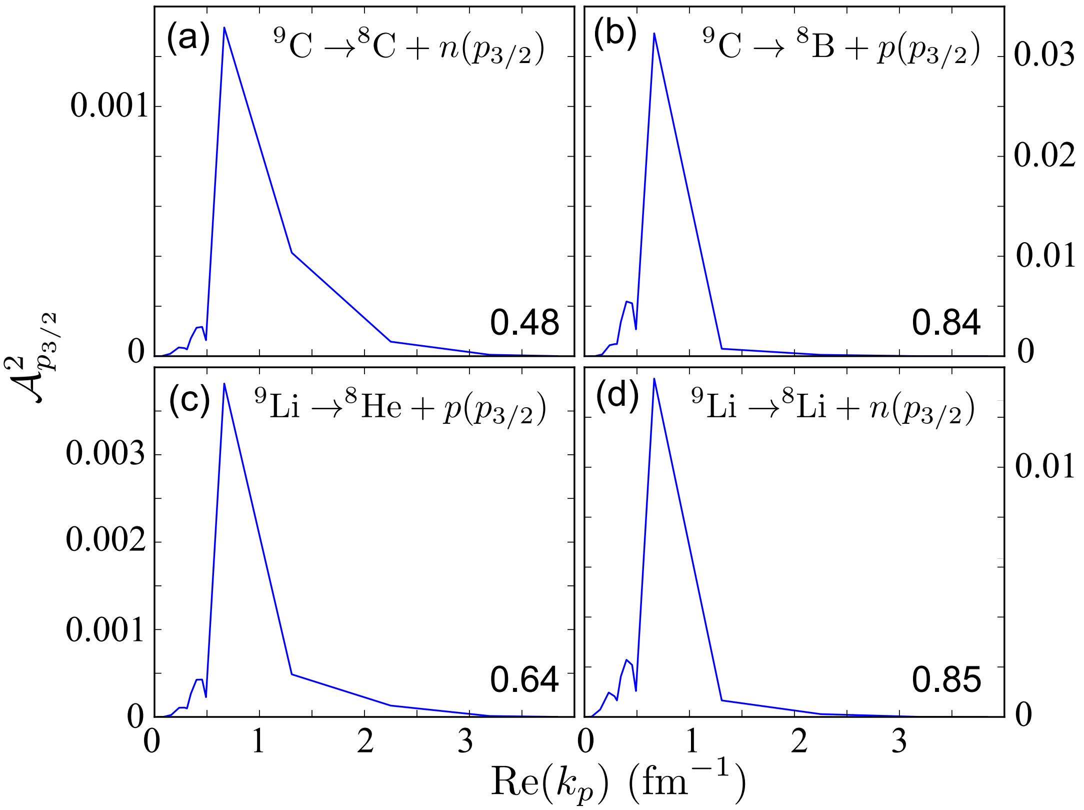


FIG. S2. Non-resonant contributions $\mathcal{A}^2_{p_{3/2}}(k_p)$ to the spectroscopic factor $\mathcal{S}^2_{p_{3/2}}$ for the knockout of nucleons from $^{9}$C (top) and $^{9}$Li (bottom) calculated in the GSM-*psd* space with $N_{\rm cont} = 4$. The numbers mark the squared spectroscopic amplitude of the $0p_{3/2}$ resonant state. The non-resonant contributions are multiplied by the integration weights as the contour integral in Eq. (1) has been discretized.

## S.III. Dominant GSM configurations

Tables S1-S4 show the dominant GSM configurations for each nucleus at *ps* and *psd* spaces. Only configurations with weights greater than 2% are listed.

TABLE S1. The dominant GSM configurations for $^8$C and $^9$C for two sets of GSM calculations. The first set of calculations was carried out in a *ps*-space with $N_{\rm cont} = 3$. The second set corresponds to *psd*-space and $N_{\rm cont} = 4$ in the continuum for $^8$C. In both cases, only two particles were allowed in the continuum for $^9$C. All energies and widths are in MeV.

| Nucleus | $J^\pi$ | $E^{\rm exp}(\Gamma^{\rm exp})$ | $E^{\rm cal}(\Gamma^{\rm cal})$ | Configuration |
|---|---|---|---|---|
| $^8$C$_{ps}$ | $0^+$ | 3.483(0.23) | 2.479(0.006) | 45% $(0p_{3/2})^4$ |
| | | | | 33% $(0p_{3/2})^3(p_{3/2}^{\rm scatt})$ |
| | | | | 13% $(0p_{3/2})^2(p_{3/2}^{\rm scatt})^2$ |
| | | | | 3% $(0p_{3/2})^2(0p_{1/2})^2$ |
| | | | | 2% $(0p_{3/2})(p_{1/2}^{\rm scatt})^3$ |
| $^9$C$_{ps}$ | $3/2^-$ | -10.742 | -10.515 | 61% $(0p_{3/2})^4_{\rm p}(0p_{3/2})_{\rm n}$ |
| | | | | 12% $(0p_{3/2})^3_{\rm p}(p_{3/2}^{\rm scatt})_{\rm p}(0p_{3/2})_{\rm n}$ |
| | | | | 10% $(0p_{3/2})^3_{\rm p}(0p_{1/2})_{\rm p}(0p_{3/2})_{\rm n}$ |
| | | | | 8% $(0p_{3/2})^2_{\rm p}(0p_{1/2})^2_{\rm p}(0p_{3/2})_{\rm n}$ |
| | | | | 2% $(0p_{3/2})^2_{\rm p}(0p_{1/2})_{\rm p}(p_{3/2}^{\rm scatt})_{\rm p}(0p_{3/2})_{\rm n}$ |
| | | | | 2% $(0p_{3/2})^2_{\rm p}(p_{3/2}^{\rm scatt})^2_{\rm p}(0p_{3/2})_{\rm n}$ |
| | $1/2^-$ | -8.56(0.1) | -7.583 | 60% $(0p_{3/2})^4_{\rm p}(0p_{3/2})_{\rm n}$ |
| | | | | 17% $(0p_{3/2})^3_{\rm p}(0p_{1/2})_{\rm p}(0p_{3/2})_{\rm n}$ |
| | | | | 9% $(0p_{3/2})^3_{\rm p}(p_{3/2}^{\rm scatt})_{\rm p}(0p_{1/2})_{\rm n}$ |
| | | | | 4% $(0p_{3/2})^2_{\rm p}(0p_{1/2})^2_{\rm p}(0p_{1/2})_{\rm n}$ |
| | | | | 3% $(0p_{3/2})^2_{\rm p}(0p_{1/2})_{\rm p}(p_{3/2}^{\rm scatt})_{\rm p}(0p_{3/2})_{\rm n}$ |
| | | | | 2% $(0p_{3/2})^3_{\rm p}(p_{3/2}^{\rm scatt})_{\rm p}(0p_{3/2})_{\rm n}$ |
| $^8$C$_{psd}$ | $0^+$ | 3.483(0.23) | 3.653(0.03) | 29% $(0p_{3/2})^4$ |
| | | | | 30% $(0p_{3/2})^3(p_{3/2}^{\rm scatt})$ |
| | | | | 21% $(0p_{3/2})^2(p_{3/2}^{\rm scatt})^2$ |
| | | | | 8% $(0p_{3/2})(p_{3/2}^{\rm scatt})^3$ |
| | | | | 3% $(0p_{3/2})^2(0p_{1/2})^2$ |
| | | | | 2% $(p_{3/2}^{\rm scatt})^4$ |
| $^9$C$_{psd}$ | $3/2^-$ | -10.742 | -9.385 | 60% $(0p_{3/2})^4_{\rm p}(0p_{3/2})_{\rm n}$ |
| | | | | 10% $(0p_{3/2})^3_{\rm p}(0p_{1/2})_{\rm p}(0p_{3/2})_{\rm n}$ |
| | | | | 9% $(0p_{3/2})^2_{\rm p}(0p_{1/2})^2_{\rm p}(0p_{1/2})_{\rm n}$ |
| | | | | 9% $(0p_{3/2})^3_{\rm p}(p_{3/2}^{\rm scatt})_{\rm p}(0p_{3/2})_{\rm n}$ |
| | | | | 2% $(0p_{3/2})^2_{\rm p}(p_{3/2}^{\rm scatt})^2_{\rm p}(0p_{3/2})_{\rm n}$ |
| | | | | 2% $(0p_{3/2})^3_{\rm p}(0p_{1/2})_{\rm p}(0p_{1/2})_{\rm n}$ |
| | $1/2^-$ | -8.56(0.1) | -5.783 | 57% $(0p_{3/2})^4_{\rm p}(0p_{1/2})_{\rm n}$ |
| | | | | 17% $(0p_{3/2})^3_{\rm p}(0p_{1/2})_{\rm p}(0p_{3/2})_{\rm n}$ |
| | | | | 8% $(0p_{3/2})^3_{\rm p}(p_{3/2}^{\rm scatt})_{\rm p}(0p_{1/2})_{\rm n}$ |
| | | | | 5% $(0p_{3/2})^2_{\rm p}(0p_{1/2})^2_{\rm p}(0p_{1/2})_{\rm n}$ |
| | | | | 3% $(0p_{3/2})^2_{\rm p}(0p_{1/2})_{\rm p}(p_{3/2}^{\rm scatt})(0p_{3/2})_{\rm n}$ |
| | | | | 2% $(0p_{3/2})^2_{\rm p}(p_{3/2}^{\rm scatt})^2_{\rm p}(0p_{1/2})_{\rm n}$ |
| | | | | 2% $(0p_{3/2})^3_{\rm p}(p_{3/2}^{\rm scatt})_{\rm p}(0p_{3/2})_{\rm n}$ |

TABLE S2. Similar as in Table S1 but for $^8$He and $^9$Li. Only two particles were allowed in the continuum for $^9$Li.

| Nucleus | $J^\pi$ | $E^{\rm exp}(\Gamma^{\rm exp})$ | $E^{\rm cal}(\Gamma^{\rm cal})$ | Configuration |
|---|---|---|---|---|
| $^8\mathrm{He}_{ps}$ | $0^+$ | -3.112 | -0.937 | 50% $(0p_{3/2})^4$ |
| | | | | 31% $(0p_{3/2})^3(p_{3/2}^{\rm scatt})$ |
| | | | | 11% $(0p_{3/2})^2(p_{3/2}^{\rm scatt})^2$ |
| | | | | 4% $(0p_{3/2})^2(0p_{1/2})^2$ |
| | | | | 2% $(0p_{3/2})(p_{3/2}^{\rm scatt})^3$ |
| $^9\mathrm{Li}_{ps}$ | $3/2^-$ | -17.045 | -16.657 | 65% $(0p_{3/2})^4_{\rm n}(0p_{3/2})_{\rm p}$ |
| | | | | 11% $(0p_{3/2})^3_{\rm n}(0p_{1/2})_{\rm n}(0p_{3/2})_{\rm p}$ |
| | | | | 9% $(0p_{3/2})^2_{\rm n}(0p_{1/2})^2_{\rm n}(0p_{3/2})_{\rm p}$ |
| | | | | 8% $(0p_{3/2})^3_{\rm n}(p_{1/2}^{\rm scatt})_{\rm n}(0p_{3/2})_{\rm p}$ |
| | $1/2^-$ | -14.354 | -13.561 | 64% $(0p_{3/2})^4_{\rm n}(0p_{1/2})_{\rm p}$ |
| | | | | 18% $(0p_{3/2})^3_{\rm n}(0p_{1/2})_{\rm n}(0p_{3/2})_{\rm p}$ |
| | | | | 6% $(0p_{3/2})^3_{\rm n}(p_{3/2}^{\rm scatt})_{\rm n}(0p_{1/2})_{\rm p}$ |
| | | | | 4% $(0p_{3/2})^2_{\rm n}(0p_{1/2})^2_{\rm n}(0p_{1/2})_{\rm p}$ |
| | | | | 2% $(0p_{3/2})^2_{\rm n}(0p_{1/2})_{\rm n}(p_{3/2}^{\rm scatt})_{\rm n}(0p_{3/2})_{\rm p}$ |
| $^8\mathrm{He}_{psd}$ | $0^+$ | -3.112 | -2.616 | 52% $(0p_{3/2})^4$ |
| | | | | 25% $(0p_{3/2})^3(p_{3/2}^{\rm scatt})$ |
| | | | | 10% $(0p_{3/2})^2(p_{3/2}^{\rm scatt})^2$ |
| | | | | 6% $(0p_{3/2})^2(0p_{1/2})^2$ |
| | | | | 2% $(0p_{3/2})(p_{3/2}^{\rm scatt})^3$ |
| $^9\mathrm{Li}_{psd}$ | $3/2^-$ | -17.045 | -18.481 | 64% $(0p_{3/2})^4_{\rm n}(0p_{3/2})_{\rm p}$ |
| | | | | 11% $(0p_{3/2})^2_{\rm n}(0p_{1/2})^2_{\rm n}(0p_{3/2})_{\rm p}$ |
| | | | | 11% $(0p_{3/2})^3_{\rm n}(0p_{1/2})_{\rm n}(0p_{3/2})_{\rm p}$ |
| | | | | 4% $(0p_{3/2})^3_{\rm n}(p_{3/2}^{\rm scatt})_{\rm n}(0p_{3/2})_{\rm p}$ |
| | | | | 2% $(0p_{3/2})^3_{\rm n}(0p_{1/2})_{\rm n}(0p_{3/2})_{\rm p}$ |
| | | | | 2% $(0p_{3/2})^2_{\rm n}(p_{3/2}^{\rm scatt})^2_{\rm n}(0p_{3/2})_{\rm p}$ |
| | $1/2^-$ | -14.354 | -14.683 | 63% $(0p_{3/2})^4_{\rm n}(0p_{1/2})_{\rm p}$ |
| | | | | 18% $(0p_{3/2})^3_{\rm n}(0p_{1/2})_{\rm n}(0p_{3/2})_{\rm p}$ |
| | | | | 6% $(0p_{3/2})^2_{\rm n}(0p_{1/2})^2_{\rm n}(0p_{1/2})_{\rm p}$ |
| | | | | 4% $(0p_{3/2})^3_{\rm n}(p_{3/2}^{\rm scatt})_{\rm n}(0p_{1/2})_{\rm p}$ |
| | | | | 2% $(0p_{3/2})^2_{\rm n}(p_{3/2}^{\rm scatt})^2_{\rm n}(0p_{1/2})_{\rm p}$ |

TABLE S3. Similar as in Table S2 but for $^8$B and $^9$C.

| Nucleus | $J^\pi$ | $E^{\mathrm{exp}}(\Gamma^{\mathrm{exp}})$ | $E^{\mathrm{cal}}(\Gamma^{\mathrm{cal}})$ | Configuration |
|---|---|---|---|---|
| $^8\mathrm{B}_{ps}$ | $2^+$ | -9.442 | -8.970 | 53% $(0p_{3/2})^3_{\mathrm{p}}(0p_{3/2})_{\mathrm{n}}$<br>13% $(0p_{3/2})^2_{\mathrm{p}}(p^{\mathrm{scatt}}_{3/2})_{\mathrm{p}}(0p_{3/2})_{\mathrm{n}}$<br>11% $(0p_{3/2})^2_{\mathrm{p}}(0p_{1/2})_{\mathrm{p}}(0p_{3/2})_{\mathrm{n}}$<br>8% $(0p_{3/2})^3_{\mathrm{p}}(0p_{1/2})_{\mathrm{n}}$<br>3% $(0p_{3/2})^2_{\mathrm{p}}(0p_{1/2})_{\mathrm{p}}(0p_{1/2})_{\mathrm{n}}$<br>3% $(0p_{3/2})_{\mathrm{p}}(0p_{1/2})^2_{\mathrm{p}}(0p_{3/2})_{\mathrm{n}}$<br>2% $(0p_{3/2})_{\mathrm{p}}(0p_{1/2})_{\mathrm{p}}(p^{\mathrm{scatt}}_{3/2})_{\mathrm{p}}(0p_{3/2})_{\mathrm{n}}$<br>2% $(0p_{3/2})^2_{\mathrm{p}}(p^{\mathrm{scatt}}_{3/2})_{\mathrm{p}}(0p_{1/2})_{\mathrm{n}}$ |
| $^9\mathrm{C}_{ps}$ | $3/2^-$ | -10.742 | -10.515 | 61% $(0p_{3/2})^4_{\mathrm{p}}(0p_{3/2})_{\mathrm{n}}$<br>12% $(0p_{3/2})^3_{\mathrm{p}}(p^{\mathrm{scatt}}_{3/2})_{\mathrm{p}}(0p_{3/2})_{\mathrm{n}}$<br>10% $(0p_{3/2})^3_{\mathrm{p}}(0p_{1/2})_{\mathrm{p}}(0p_{3/2})_{\mathrm{n}}$<br>8% $(0p_{3/2})^2_{\mathrm{p}}(0p_{1/2})^2_{\mathrm{p}}(0p_{3/2})_{\mathrm{n}}$<br>2% $(0p_{3/2})^2_{\mathrm{p}}(0p_{1/2})_{\mathrm{p}}(p^{\mathrm{scatt}}_{3/2})_{p}(0p_{3/2})_{\mathrm{n}}$<br>2% $(0p_{3/2})^2_{\mathrm{p}}(p^{\mathrm{scatt}}_{3/2})^2_{p}(0p_{3/2})_{\mathrm{n}}$ |
| | $1/2^-$ | -8.56(0.1) | -7.583 | 60% $(0p_{3/2})^4_{\mathrm{p}}(0p_{3/2})_{\mathrm{n}}$<br>17% $(0p_{3/2})^3_{\mathrm{p}}(0p_{1/2})_{\mathrm{p}}(0p_{3/2})_{\mathrm{n}}$<br>9% $(0p_{3/2})^3_{\mathrm{p}}(p^{\mathrm{scatt}}_{3/2})_{\mathrm{p}}(0p_{1/2})_{\mathrm{n}}$<br>4% $(0p_{3/2})^2_{\mathrm{p}}(0p_{1/2})^2_{\mathrm{p}}(0p_{1/2})_{\mathrm{n}}$<br>3% $(0p_{3/2})^2_{\mathrm{p}}(0p_{1/2})_{\mathrm{p}}(p^{\mathrm{scatt}}_{3/2})_{\mathrm{p}}(0p_{3/2})_{\mathrm{n}}$<br>2% $(0p_{3/2})^3_{\mathrm{p}}(p^{\mathrm{scatt}}_{3/2})_{\mathrm{p}}(0p_{3/2})_{\mathrm{n}}$ |
| $^8\mathrm{B}_{psd}$ | $2^+$ | -9.442 | -12.817 | 52% $(0p_{3/2})^3_{\mathrm{p}}(0p_{3/2})_{\mathrm{n}}$<br>9% $(0p_{3/2})^2_{\mathrm{p}}(p^{\mathrm{scatt}}_{3/2})_{\mathrm{p}}(0p_{3/2})_{\mathrm{n}}$<br>9% $(0p_{3/2})^2_{\mathrm{p}}(0p_{1/2})_{\mathrm{p}}(0p_{3/2})_{\mathrm{n}}$<br>4% $(0p_{3/2})^3_{\mathrm{p}}(0p_{1/2})_{\mathrm{n}}$<br>3% $(0p_{3/2})^2_{\mathrm{p}}(0p_{1/2})_{\mathrm{p}}(0p_{1/2})_{\mathrm{n}}$<br>3% $(0p_{3/2})_{\mathrm{p}}(0d_{5/2})^2_{\mathrm{p}}(0d_{5/2})_{\mathrm{n}}$<br>3% $(0p_{3/2})_{\mathrm{p}}(0d_{5/2})^2_{\mathrm{p}}(0p_{3/2})_{\mathrm{n}}$<br>3% $(0p_{3/2})_{\mathrm{p}}(0p_{1/2})^2_{\mathrm{p}}(0p_{3/2})_{\mathrm{n}}$ |
| $^9\mathrm{C}_{psd}$ | $3/2^-$ | -10.742 | -9.385 | 60% $(0p_{3/2})^4_{\mathrm{p}}(0p_{3/2})_{\mathrm{n}}$<br>10% $(0p_{3/2})^3_{\mathrm{p}}(0p_{1/2})_{\mathrm{p}}(0p_{3/2})_{\mathrm{n}}$<br>9% $(0p_{3/2})^2_{\mathrm{p}}(0p_{3/2})^2_{\mathrm{p}}(0p_{1/2})_{\mathrm{n}}$<br>9% $(0p_{3/2})^3_{\mathrm{p}}(p^{\mathrm{scatt}}_{3/2})_{\mathrm{p}}(0p_{3/2})_{\mathrm{n}}$<br>2% $(0p_{3/2})^3_{\mathrm{p}}(0p_{1/2})_{\mathrm{p}}(0p_{1/2})_{\mathrm{n}}$<br>2% $(0p_{3/2})^2_{\mathrm{p}}(p^{\mathrm{scatt}}_{3/2})^2_{\mathrm{p}}(0p_{3/2})_{\mathrm{n}}$ |
| | $1/2^-$ | -8.56(0.1) | -5.783 | 57% $(0p_{3/2})^4_{\mathrm{p}}(0p_{1/2})_{\mathrm{n}}$<br>17% $(0p_{3/2})^3_{\mathrm{p}}(0p_{1/2})_{\mathrm{p}}(0p_{3/2})_{\mathrm{n}}$<br>8% $(0p_{3/2})^3_{\mathrm{p}}(p^{\mathrm{scatt}}_{3/2})_{\mathrm{p}}(0p_{1/2})_{\mathrm{n}}$<br>5% $(0p_{3/2})^2_{\mathrm{p}}(0p_{1/2})^2_{\mathrm{p}}(0p_{1/2})_{\mathrm{n}}$<br>3% $(0p_{3/2})^2_{\mathrm{p}}(0p_{1/2})_{\mathrm{p}}(p^{\mathrm{scatt}}_{3/2})(0p_{3/2})_{\mathrm{n}}$<br>2% $(0p_{3/2})^2_{\mathrm{p}}(p^{\mathrm{scatt}}_{3/2})^2_{\mathrm{p}}(0p_{1/2})_{\mathrm{n}}$<br>2% $(0p_{3/2})^3_{\mathrm{p}}(p^{\mathrm{scatt}}_{3/2})_{\mathrm{p}}(0p_{3/2})_{\mathrm{n}}$ |

TABLE S4. Similar as in Table S1 but for $^{8,9}$Li.

| Nucleus | $J^\pi$ | $E^{\mathrm{exp}}(\Gamma^{\mathrm{exp}})$ | $E^{\mathrm{cal}}(\Gamma^{\mathrm{cal}})$ | Configuration |
|---|---|---|---|---|
| $^8\mathrm{Li}_{ps}$ | $2^+$ | -12.982 | -12.446 | 57% $(0p_{3/2})^3_n(0p_{3/2})_p$ |
| | | | | 12% $(0p_{3/2})^2_n(0p_{1/2})_n(0p_{3/2})_p$ |
| | | | | 9% $(0p_{3/2})^2_n(p^{\mathrm{scatt}}_{3/2})_n(0p_{3/2})_p$ |
| | | | | 8% $(0p_{3/2})^3_n(0p_{1/2})_p$ |
| | | | | 3% $(0p_{3/2})^2_n(p_{1/2})_n(0p_{1/2})_p$ |
| | | | | 3% $(0p_{3/2})_n(p_{1/2})^2_n(0p_{1/2})_p$ |
| | | | | 2% $(0p_{3/2})_n(p_{1/2})_n(p^{\mathrm{scatt}}_{3/2})_n(0p_{3/2})_p$ |
| $^9\mathrm{Li}_{ps}$ | $3/2^-$ | -17.045 | -16.657 | 65% $(0p_{3/2})^4_\mathrm{n}(0p_{3/2})_\mathrm{p}$ |
| | | | | 11% $(0p_{3/2})^3_\mathrm{n}(0p_{1/2})_\mathrm{n}(0p_{3/2})_\mathrm{p}$ |
| | | | | 9% $(0p_{3/2})^2_\mathrm{n}(0p_{1/2})^2_\mathrm{n}(0p_{3/2})_\mathrm{p}$ |
| | | | | 8% $(0p_{3/2})^3_\mathrm{n}(p^{\mathrm{scatt}}_{1/2})_\mathrm{n}(0p_{3/2})_\mathrm{p}$ |
| | $1/2^-$ | -14.354 | -13.561 | 64% $(0p_{3/2})^4_\mathrm{n}(0p_{1/2})_\mathrm{p}$ |
| | | | | 18% $(0p_{3/2})^3_\mathrm{n}(0p_{1/2})_\mathrm{n}(0p_{3/2})_\mathrm{p}$ |
| | | | | 6% $(0p_{3/2})^3_\mathrm{n}(p^{\mathrm{scatt}}_{3/2})_\mathrm{n}(0p_{1/2})_\mathrm{p}$ |
| | | | | 4% $(0p_{3/2})^2_\mathrm{n}(0p_{1/2})^2_\mathrm{n}(0p_{1/2})_\mathrm{p}$ |
| | | | | 2% $(0p_{3/2})^2_\mathrm{n}(0p_{1/2})_\mathrm{n}(p^{\mathrm{scatt}}_{3/2})_\mathrm{n}(0p_{3/2})_\mathrm{p}$ |
| $^8\mathrm{Li}_{psd}$ | $2^+$ | -12.982 | -18.140 | 56% $(0p_{3/2})^3_n(0p_{3/2})_p$ |
| | | | | 9% $(0p_{3/2})^2_n(0p_{1/2})_n(0p_{3/2})_p$ |
| | | | | 5% $(0p_{3/2})^3_n(0p_{1/2})_p$ |
| | | | | 4% $(0p_{3/2})^2_n(0p_{1/2})_n(0p_{1/2})_p$ |
| | | | | 4% $(0p_{3/2})^2_n(p^{\mathrm{scatt}}_{3/2})_n(0p_{3/2})_p$ |
| | | | | 3% $(0p_{3/2})^2_n(0d_{5/2})_n(0d_{5/2})_p$ |
| | | | | 3% $(0p_{3/2})_n(0d_{5/2})^2_n(0p_{3/2})_p$ |
| | | | | 3% $(0p_{3/2})_n(0p_{1/2})^2_n(0p_{3/2})_p$ |
| | | | | 2% $(0p_{3/2})^2_n(p^{\mathrm{scatt}}_{3/2})_n(p^{\mathrm{scatt}}_{3/2})_p$ |
| $^9\mathrm{Li}_{psd}$ | $3/2^-$ | -17.045 | -18.481 | 64% $(0p_{3/2})^4_\mathrm{n}(0p_{3/2})_\mathrm{p}$ |
| | | | | 11% $(0p_{3/2})^2_\mathrm{n}(0p_{1/2})^2_\mathrm{n}(0p_{3/2})_\mathrm{p}$ |
| | | | | 11% $(0p_{3/2})^3_\mathrm{n}(0p_{1/2})_\mathrm{n}(0p_{3/2})_\mathrm{p}$ |
| | | | | 4% $(0p_{3/2})^3_\mathrm{n}(p^{\mathrm{scatt}}_{3/2})_\mathrm{n}(0p_{3/2})_\mathrm{p}$ |
| | | | | 2% $(0p_{3/2})^3_\mathrm{n}(0p_{1/2})_\mathrm{n}(0p_{3/2})_\mathrm{p}$ |
| | | | | 2% $(0p_{3/2})^2_\mathrm{n}(p^{\mathrm{scatt}}_{3/2})^2_\mathrm{n}(0p_{3/2})_\mathrm{p}$ |
| | $1/2^-$ | -14.354 | -14.683 | 63% $(0p_{3/2})^4_\mathrm{n}(0p_{1/2})_\mathrm{p}$ |
| | | | | 18% $(0p_{3/2})^3_\mathrm{n}(0p_{1/2})_\mathrm{n}(0p_{3/2})_\mathrm{p}$ |
| | | | | 6% $(0p_{3/2})^2_\mathrm{n}(0p_{1/2})^2_\mathrm{n}(0p_{1/2})_\mathrm{p}$ |
| | | | | 4% $(0p_{3/2})^3_\mathrm{n}(p^{\mathrm{scatt}}_{3/2})_\mathrm{n}(0p_{1/2})_\mathrm{p}$ |
| | | | | 2% $(0p_{3/2})^2_\mathrm{n}(p^{\mathrm{scatt}}_{3/2})^2_\mathrm{n}(0p_{1/2})_\mathrm{p}$ |
